# Supplementary material for: On The Reachability Problem for Recursive Hybrid Automata with One and Two Players
Source: arXiv:1406.7289 source file (2014-08-15)
Supplement: Supplementary file 1 [file appendix.tex]

% \section{Detailed Undecidability Proofs}
% \input{rha-2.tex}
% \input{tb-rta-5.tex}
% \input{rha-3.tex}
% \input{tb-rha-14.tex}

% {Decidability of 2 stopwatch RHA}
% \input{dec-rha.tex}
% \input{dec-ref-full-app.tex}
